# Supplementary material for: Self-expressive Dictionary Learning for Dynamic 3D Reconstruction
Source: arXiv:1605.06863 source file (2016-05-22)
Supplement: Supplementary file 1 [file supp.tex]

\clearpage
\onecolumn
\begin{center}
\textbf{\large Supplemental Materials: Title for main text}
\end{center}

\section{Section 1}
Copy and paste your Supplemental Materials text here \cite{S_RefA}, blah, blah, blah, blah, blah, blah, ...
\begin{equation}
  i\hbar\frac{\partial}{\partial t}\psi(x,t) = -\frac{\hbar^2}{2m}\frac{\partial^2}{\partial x^2}\psi(x,t) + V(x,t) \psi(x,t)
\end{equation}
