# Supplementary material for: Self-expressive Dictionary Learning for Dynamic 3D Reconstruction
Source: arXiv:1605.06863 source file (2016-05-22)

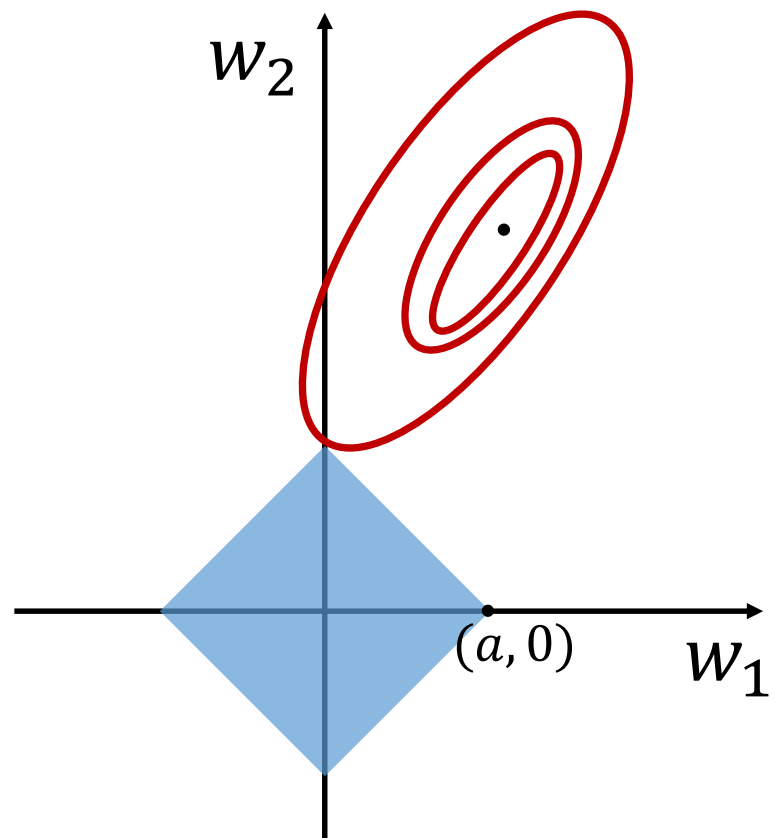

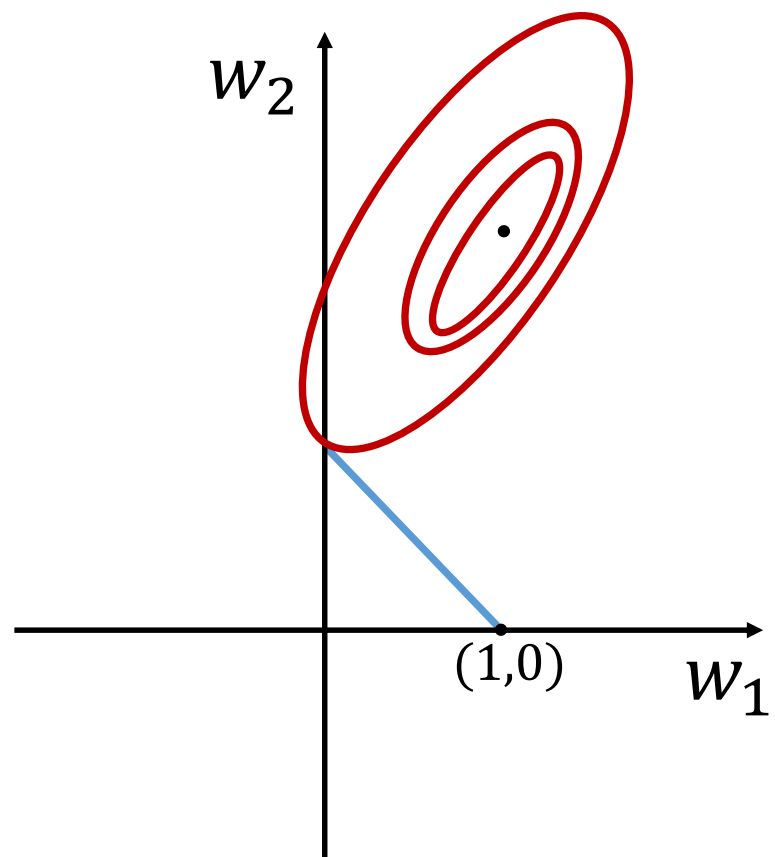

Supplement: Supplementary file 2 [file sum_to_1.pdf]
